# Supplementary material for: On the essential minimum of Faltings' height
Source: arXiv:1609.00071 ancillary file (2017-04-12)
Supplement: Supplementary file 1 [file EllipticCurvesOfSmallHeight.pdf]

# EllipticCurvesOfSmallHeight

José Ignacio Burgos Gil,<sup>\*</sup> Ricardo Menares & Juan Rivera-Letelier<sup>†</sup>

August 31, 2016

## Abstract

We describe a procedure using a SAGE worksheet that allowed us to do the numerical experiments mentioned in our manuscript [BMRL]

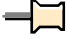

We first import the extra packages we need: optimize and complex\_roots.

```
import scipy
from scipy import optimize
K, t = PolynomialRing(QQ, 't').objgen()
from sage.rings.polynomial.complex_roots import complex_roots
```

We define the basic functions we will use. The Dedekind  $\eta$  function is already implemented in SAGE with arbitrary precision. It is given by

$$\eta(\tau) = q^{1/24} \prod_{k=1}^{\infty} (1 - q^k)$$

where  $q = \exp(2\pi i\tau)$ .

The function  $\Delta$  is given by  $\Delta(\tau) = \eta^{24}(\tau)$ .

The function  $j$  is given by

$$j(\tau) = \frac{(w+16)^3}{w},$$

where

$$w = \left( \frac{\sqrt{2}\eta(2\tau)}{\eta(\tau)} \right)^{24}.$$

Recall that  $\Delta$  determines a section of the line bundle  $\mathcal{O}(1)$  on the modular curve  $\mathbb{P}^1$ .

We force the functions we define to work with float numbers instead of working symbolically to increase speed.

```
Pi=N(pi)
# delta function
def Delta (z):
    h=z.eta()
    return h^24

# j-invariant.
def j(z):
    z2=2.*z
    u=z2.eta()
    v=z.eta()
    w=(sqrt(2.)*u/v)^24
    return (w+16)^3/w
```

---

<sup>\*</sup>Burgos was partially supported by the MINECO research projects MTM2013-42135-P and ICMAT Severo Ochoa SEV-2015-0554.

<sup>†</sup>Rivera-Letelier was partially supported by FONDECYT grant 1141091.

The inverse of  $j$  is given in terms of hypergeometric functions. Namely

$$j^{-1}(z) = i \frac{{}_2F_1(1/6, 5/6, 1, 1 - \alpha)}{{}_2F_1(1/6, 5/6, 1, \alpha)},$$

where  $\alpha$  is a root of the quadratic equation

$$4z\alpha(1 - \alpha) = 1728.$$

<div>  
</div>

```
# Inverse of j
def jinv(z):
    if z == 0:
        return .5+I*sqrt(3.)/2
    z1=1.-1728/z
    w=(1+z1.sqrt())/2
    h1=hypergeometric([1/6,5/6],[1],w.real()+I*w.imag())
    h2=hypergeometric([1/6,5/6],[1],1-w.real()-I*w.imag())
    return I*h2/h1
```

The Green function associated to the Petersson metric (with the normalization we use) in the upper half plane is given by

$$g_H(\tau) = g_\infty(\tau)/12 = -\log(\|\Delta\|_{Pet}^2)/24 = -\log(4\pi\Im(\tau))/2 - \log(|\eta(\tau)|^2).$$

The Green function on the projective line is given by

$$g(z) = g_H(j^{-1}(z)).$$

```
# Green function in the upper half plane
def green_H(z):
    y=imag(4*Pi*z)
    r=norm(eta(z))
    green=-log(y*r*r)/2
    return green

# Green function in the projective line
def green(z):
    return green_H(jinv(z))

# We plot the green function in a neighbourhood of the point zero to see
# that the minimum is attained at this point
A=plot3d(lambda x,y : float(green(x+y*i)),(-3000,3000),(-3000,3000))
A.show()
```

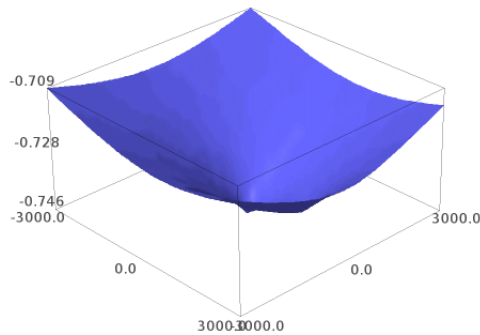

Given an irreducible polynomial, all its roots have the same height. We call it the height of the polynomial. The next function computes the height of an irreducible polynomial with integral coefficients. Note that, if the polynomial is monic and has integral coefficients, then the non-Archimedean contributions to the height vanish.

```
def height_pol(p):
    h=0
    d=p.degree()
    for P in complex_roots(p):
        z=P[0].center()
        z1=z.real()+I*z.imag()
        h=h+green(z1)
    return h/d
```

```
height_pol(t)
```

```
-0.748752485503338
```

As an example, we compute the height of the first 30 cyclotomic polynomials, order them by height and show the first 6.

```
h_cyc=[]
for ii in range(30):
    p=cyclotomic_polynomial(ii+1)
    h=height_pol(p)
    h_cyc=h_cyc+[[p,h]]
def second(a,b):
    if a[1] == b[1]:
        return int(0)
    if a[1] > b[1]:
        return int(1)
    if a[1] < b[1]:
        return int(-1)
h_cyc.sort(cmp=second)
h_cyc[:6]

[[x - 1, -0.748628177398873],
 [x^2 - x + 1, -0.748625170543322],
 [x^4 - x^3 + x^2 - x + 1, -0.748623668322015],
 [x^6 - x^5 + x^4 - x^3 + x^2 - x + 1, -0.748623167581391],
 [x^8 - x^7 + x^5 - x^4 + x^3 - x + 1, -0.748622917512343],
 [x^10 - x^9 + x^8 - x^7 + x^6 - x^5 + x^4 - x^3 + x^2 - x + 1,
 -0.748622766988892]]
```

We now compute upper bounds for the essential minimum. The integral of the Green function against the equilibrium measure of a set of capacity one (with respect to infinity) is an upper bound for the essential minimum. The first example of a set of capacity one is the unit circle.

```
def g_circ(theta):
    z=exp(2*Pi*theta*I)
    return green(z)

integral_numerical(g_circ,0,1)[0]

-0.7486221661001435
```

We will now search for other sets of capacity one. The easiest way to parametrize such sets is by the parametrization:

$$h(z) = 1/z + a + bz + cz^2 + \dots$$

where  $z$  runs on the unit circle. Moreover, the image of the uniform probability measure on the circle gives the equilibrium measure on the set.

We use a list for the coefficients  $a, b, \dots$  so we can study different kind of curves. We start by defining a parametrization of the curve and a function that computes the integral.

```
def g_circ_2(theta,AA):
    z0=exp(2*Pi*theta*I)
    z=1/z0
    zk=1
```

```

for a in AA:
    z=z+a*zk
    zk=zk*z0
return green(z)

def integ_jordan(AA):
    integ=integral_numerical(lambda x : g_circ_2(x,AA),0,1)[0]
    return integ

```

As an example we compute the upper bound given by the circle translated by .2.

```

integ_jordan([.2])
-0.748622784920585

```

We obtain a better upper bound. We now optimize the upper bound.

```

AA=[.2]
optimize.fmin(integ_jordan,AA)
Optimization terminated successfully.
    Current function value: -0.748623
    Iterations: 8
    Function evaluations: 16
array([ 0.2053125])

```

```

AA=[ 0.2053125]
integ_jordan(AA)
-0.7486227853380368

```

So we have obtained a slightly upper bound.

We now try to improve the bound by adding an excentricity parameter.

```

AA=[ 0.2053125,0]
optimize.fmin(integ_jordan,AA)
Optimization terminated successfully.
    Current function value: -0.748623
    Iterations: 29
    Function evaluations: 54
array([ 0.20726323,  0.01433166])

```

```

AA=[ 0.20726323,  0.01433166]
integ_jordan(AA)
-0.7486227882980458

```

We now add more parameters to see if we can still improve the upper bound.

```

AA=[ 0.20732052,  0.01436212,0,0,0]
optimize.fmin(integ_jordan,AA)
Optimization terminated successfully.
    Current function value: -0.748623
    Iterations: 34
    Function evaluations: 57
array([ 2.07247955e-01,  1.43666464e-02,  3.12243672e-04,
        -1.34314267e-05, -9.66426512e-06])

```

```

AA=[ 2.07247955e-01,  1.43666464e-02,  3.12243672e-04, -1.34314267e-05, -9.66426512e-06]
integ_jordan(AA)
-0.7486227882996481

```

```

bound=-0.7486227882996481

```

The improvement of the upper bound is negligible. As a conclusion an upper bound for the essential minimum is given by

$$B = -0.748622788299$$

Note also that the set of values of the height of algebraic points above this bound is dense.

We now search systematically polynomials with low height. After crunching hundreds of millions of polynomials of degree lower or equal that 10 with PARI, we have found many polynomials whose height is lower than the previous upper bound. These are stored in the file "low\_height\_pol.txt". To load it with the next set of instructions the file should be in the directory where sage has been invoked.

```
filename=DIR+"/low_height_pol.txt"
file=open(filename,'r')

line=file.readline()
small_pol=[]
while len(line)>0:
    p=K(line)
    line=file.readline()
    h=float(line)
    small_pol=small_pol+[[p,h]]
    line=file.readline()

file.close()
```

We have found 124 polynomials up to degree 10. The list is fairly complete up to degree 6 but there can be other polynomials of degree up to 10, as well as lots of polynomials of higher degree.

```
len(small_pol)

124

small_pol[:10]

[[t, -0.748752485503338],
 [t - 1, -0.748628177398873],
 [t^2 - t + 1, -0.748625170543322],
 [t^4 - t^3 + t^2 - t + 1, -0.748623668322015],
 [t^8 - 2*t^7 + 2*t^6 - t^5 + t^4 - t^3 + t^2 - t + 1, -0.748623301572786],
 [t^6 - 2*t^5 + 2*t^4 - 2*t^3 + 2*t^2 - t + 1, -0.748623211455762],
 [t^9 - 2*t^8 + 2*t^7 - t^6 + t^4 - t^3 + t^2 - t + 1, -0.748623198923641],
 [t^10 - 3*t^9 + 4*t^8 - 3*t^7 + t^6 + t^5 - t^4 + t^2 - t + 1,
  -0.748623173387089],
 [t^8 - 2*t^7 + 2*t^6 - t^5 + t^3 - t + 1, -0.748623170365597],
 [t^6 - t^5 + t^4 - t^3 + t^2 - t + 1, -0.748623167581391]]

small_pol[120:]

[[t^9 - 2*t^8 + t^7 - t^5 + t^4 - t^2 + t - 1, -0.748622791551555],
 [t^10 - 2*t^9 + 2*t^8 - 3*t^7 + 3*t^6 - 3*t^5 + 3*t^4 - 2*t^3 + 2*t^2 - t + 1,
  -0.748622791313374],
 [t^10 - 2*t^9 + t^8 + t^2 - t + 1, -0.748622789007739],
 [t^9 - 3*t^8 + 4*t^7 - 4*t^6 + 4*t^5 - 3*t^4 + 2*t^3 - 2*t^2 + t - 1,
  -0.748622788563659]]
```

The next task is to find lower bounds for the essential minimum and to prove that certain values of the height are isolated.

The next function computes

$$\min_{z \in \mathbb{P}^1} (g(z) - A \log |z|) = -\log(\max \|s_A(z)\|_{Pet}),$$

where  $s_A$  is the section

$$s_A = \Delta^{1/12} j^A.$$

For technical reasons, the function returns the oposite of the sought value.

```
def sup_pol1(A):
    if min(A)<0:
        return 10
    g_s= lambda BB: green(BB[0]+i*BB[1])-A[0]*log(abs((BB[0]+i*BB[1])))
    op=optimize.fmin(g_s, [0,1],ftol=10^-10,disp=0,maxfun=1000,maxiter=1000)
    return -g_s(op)
```

We now look for the value of  $A$  that gives us the minimal sup norm. That is, we look for

$$\max_A \min_{z \in \mathbb{P}^1} -\log(\|s_A(z)\|_{Pet}).$$

```
AA=[.0001]
optimize.fmin(sup_pol1,AA,ftol=10^-10))
Optimization terminated successfully.
    Current function value: 0.748628
    Iterations: 9
    Function evaluations: 18
array([ 8.09375000e-05])

-sup_pol1([ 8.09375000e-05])
-0.7486281774201359
```

The best parameter  $A$  obtained is 0.0000809375. We can compare this value with the theoretical best value

$$A = \partial_x g(1) = \frac{E_2^*(\tau_1)E_4(\tau_1)}{12E_6(\tau_1)},$$

where  $j(\tau_1) = 1$ .

```
# Funcion psi, derivative of g in 1.
def psi(z):
    y=z.imag()
    q=(2*Pi*I*z).exp()
    EEcuatro=240*(1/240 + q + 9*q^2 + 28*q^3 + 73*q^4 + 126*q^5\
+ 252*q^6 + 344*q^7 + 585*q^8 + 757*q^9 + 1134*q^10 + 1332*q^11 +\
2044*q^12 + 2198*q^13 + 3096*q^14 + 3528*q^15 + 4681*q^16 + 4914*q^17\
+ 6813*q^18 + 6860*q^19)
    EEseis=-504*(-1/504 + q + 33*q^2 + 244*q^3 + 1057*q^4 + 3126*q^5 +\
8052*q^6 + 16808*q^7 + 33825*q^8 + 59293*q^9 + 103158*q^10 +\
161052*q^11 + 257908*q^12 + 371294*q^13 + 554664*q^14 + 762744*q^15 +\
1082401*q^16 + 1419858*q^17 + 1956669*q^18 + 2476100*q^19)
    EEdos=-24*(-1/24 + q + 3*q^2 + 4*q^3 + 7*q^4 + 6*q^5 + 12*q^6 +\
8*q^7 + 15*q^8 + 13*q^9 + 18*q^10 + 12*q^11 + 28*q^12 + 14*q^13 +\
24*q^14 + 24*q^15 + 31*q^16 + 18*q^17 + 39*q^18 + 20*q^19)
    p=(EEdos-(3/(Pi*y)))*EEcuatro/EEseis
    return p/12

tau1=jinv(1)
print psi(tau1)
0.0000808904747082571 - 1.22650370762423e-18*I
```

The difference between the theoretical value  $A_t = 0.0000808905$  and the experimental one  $A_e = 0.0000809375$  lies in the tolerance of the optimization.

```
AA=[ 0.0000808904747082515]
-sup_pol1(AA)
-0.7486281773988621
```

The difference lies in the tenth decimal digit that was the stated tolerance.

This implies that the height of any point different from zero and infinity is bigger than  $-0.748628177398871$  which is precisely the height of the point 1.

```
green(0)
-0.748752485503337
```

```
green(1)
-0.748628177398873
```

We plot the function  $-\log(\|s_{A_e}\|_{Pet})$ . Observe that there is a single minimum at the point 1.

```
AA=[0.000080889992 ]
A=plot3d(lambda x,y: min_symbolic(-0.74862,green(x+i*y)-AA[0]*(x+i*y).abs().log()),(-1.6,1.6),(-1.6,1.6),a
show(A)
```

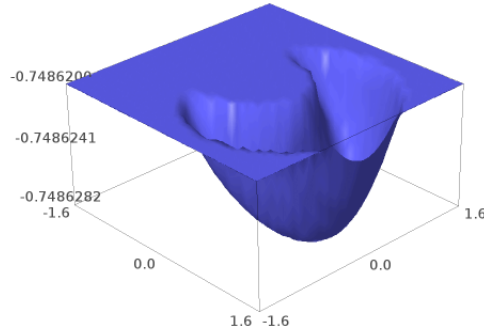

We now repeat the whole process with sections of the form

$$s_A = \Delta^{1/12} j^{A[0]} (j-1)^{A[1]}.$$

This will give an experimental lower bound for the height of any point different from 0, 1,  $\infty$ .

In order to iterate this process we will use a global variable "AA" that keeps the coefficients of the section we want to work with. For instance if  $AA = [A[0], A[1]]$  we will consider the previously mentioned section. If AA has more components we will be adding more polynomials from the list of low height polynomials.

```
def green_s(BB):
    z=BB[0]+I*BB[1]
    r=green(z)
    for j in range(len(AA)):
        p=small_pol[j][0]
        r=r-AA[j]*log(abs(p(z)))
    return r
```

The next function updates the global variable AA and computes the minimum of the corresponding Green function. Since the Green functions will have several local minima, we use different seed points to find the global minima.

```
seeds=[exp(2*Pi*I/6)]

def sup_pols(A):
    global AA
    if min(A)<0:
        return 10
    AA=A
    results=[]
    for z in seeds:
        x1=real(z)
        y1=imag(z)
        op=optimize.fmin(green_s, [x1,y1],disp=0)
        val=-green_s(op)
        results=results+[val]
    return max(results)
```

Finally we optimize with respect to the parameters in AA.

```

AA=[0.000080889992, 0]
optimize.fmin(sup_pols,AA,ftol=1e-9)
Optimization terminated successfully.
      Current function value: 0.748625
      Iterations: 18
      Function evaluations: 33
array([ 8.09845574e-05,  6.16216660e-06])

AA=[ 8.09845574e-05,  6.16216660e-06 ]
B=-sup_pols(AA)
print B
-0.7486251715714438

```

This shows that the minimal height for a point different from  $0, 1, \infty$  is  $-0.74862517$ .

Since this value is strictly higher than the height of the point 1 we deduce that  $h(1)$  is an isolated value of the height. Moreover, the new minima is attained close to the point  $\rho = \exp(\pi i/3) = 1/2 + i\sqrt{3}/2$ , who is a solution of the equation  $t^2 - t + 1$ , that is the next polynomial in our list. So we have a clear candidate to be the next isolated value.

```

green(.5+I*sqrt(3.)/2)
-0.748625170543322

```

Thus a candidate for the next minimal value of the height is  $\rho$ . We again plot the function  $-\log(\|s_{A_e}\|_{Pet})$  to see that it has two minima in  $\rho$  and  $\bar{\rho}$ .

```

AA=[ 8.09845574e-05,  6.16216660e-06 ]
A=plot3d(lambda x,y: min_symbolic(bound,green(x+I*y)-AA[0]*(x+I*y).abs().log()-AA[1]*(x-1+I*y).abs().log())
show(A)

```

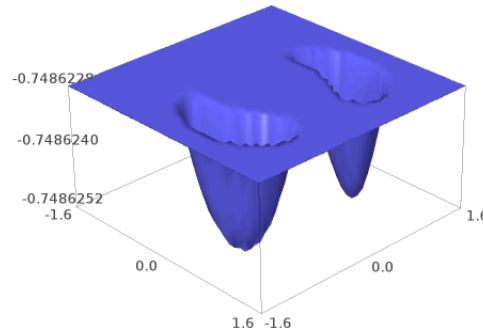

To check experimentally that  $\rho$  gives us another isolated value of the height we repeat the process with sections of the form

$$s_A = \Delta^{1/12} j^{A[0]} (j-1)^{A[1]} (j^2 - j + 1)^{A[2]}.$$

In this case we have to be careful because the function to optimize has several local minima and we have to be sure to control all of them. For this we add another seed.

```

AA=[ 8.09845574e-05,  6.16216660e-06 , 0.]
seeds=[exp(2*Pi*I/8),I]
optimize.fmin(sup_pols,AA,ftol=10^(-10))
Optimization terminated successfully.
      Current function value: 0.748624
      Iterations: 53
      Function evaluations: 97
array([ 7.98200440e-05,  4.43930324e-06,  2.44989321e-06])

```



```
AA=[ 7.98200440e-05, 4.43930324e-06, 2.44989321e-06]
B=-sup_pols(AA)
print B
-0.7486238645983615
```

We deduce that the height of any point different from  $0, 1, \infty, \rho, \bar{\rho}$  has to be bigger than  $-0.748623864557296$  showing that  $h(\rho)$  is again an isolated value. We plot the function  $-\log(\|s_{Ae}\|_{Pet})$  to see that it has the right shape.

```
A=plot3d(lambda x,y: min_symbolic(bound,green(x+I*y)-AA[0]*(x+I*y).abs().log()-AA[1]*(x-1+I*y).abs().log())
show(A)
```

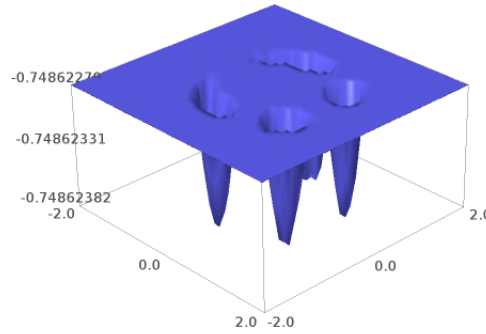

The points where the minimum is attained are close to the roots of the next polynomial on the list. In fact the height of the polynomial  $x^4 - x^3 + x^2 - x + 1$  is close to the current lower bound for the essential minimum and the roots of this polynomial are close to the points where the minimum is attained so it is a natural candidate to the next isolated value of the height.

```
complex_roots(t^4 - t^3 + t^2 - t + 1)
[(-0.309016994374948? - 0.951056516295154?*I, 1),
 (-0.309016994374948? + 0.951056516295154?*I, 1),
 (0.809016994374948? - 0.587785252292473?*I, 1),
 (0.809016994374948? + 0.587785252292473?*I, 1)]

height_pol(t^4 - t^3 + t^2 - t + 1)
-0.748623668322015
```

To check that we have another isolated value we consider sections of the form

$$s_A = \Delta^{1/12} j^{A[0]} (j-1)^{A[1]} (j^2-j+1)^{A[2]} (j^4-j^3+j^2-j+1)^{A[3]}.$$

The minimization process is more complex and we need more seeds to reach all local minima.

```
z1=exp(I*2*Pi/20)
z2=exp(I*4*Pi/15)
z3=exp(I*7*Pi/15)
z4=exp(I*11*Pi/15)
seeds=[z1,z2,z3,z4]

AA=[ 7.98200440e-05, 4.43930324e-06, 2.44989321e-06, 0]
optimize.fmin(sup_pols,AA,ftol=10^(-10))

Optimization terminated successfully.
    Current function value: 0.748624
    Iterations: 129
    Function evaluations: 226
array([ 7.80791579e-05, 3.80677028e-06, 2.36961956e-06,
 8.79532978e-07])
```

```
AA=[ 7.80791579e-05, 3.80677028e-06, 2.36961956e-06,
      8.79532978e-07]
-sup_pols(AA)
-0.7486236037646861
```

This shows experimentally that we have found another isolated value of the height. We again plot the function  $-\log(\|s_{A_e}\|_{Pet})$  to see that it has the right shape.

```
A=plot3d(lambda x,y: min_symbolic(bound,green(x+I*y)-AA[0]*(x+I*y).abs().log()\
-AA[1]*(x-1+I*y).abs().log()\
-AA[2]*((x+I*y)^2-(x+I*y)+1).abs().log()\
-AA[3]*((x+I*y)^4-(x+I*y)^3+(x+I*y)^2-(x+I*y)+1).abs().log()
),(-2,2),(-2,2),adaptative=True)
show(A)
```

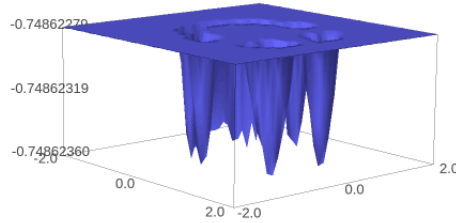

Every time the optimization process will be more time consuming. To increase performance we construct a polynomial of degree 6 that approximates the Green function in the region of interest. Since the Green function has an elliptic singularity of degree 3 we approximate the function  $g(z^3)$ .

```
var('x1,x2,a1,a2,a3,a4,a5,a6,a7,a8,a9,a10,a11,a12,a13,a14,a15')
base=green(0)
model(x1,x2)=(base+a1*x1+a2*x1^2+a3*x2^2+a4*x1^3+a5*x1*x2^2+a6*x1^4+a7*x1^2*x2^2+a8*x2^4
+a9*x1^5+a10*x1^3*x2^2+a11*x1*x2^4+a12*x1^6+a13*x1^4*x2^2+a14*x1^2*x2^4+a15*x2^6)
data=[(k/30-2., j/30-2., green((k/30-2.+1j*(j/30-2.))^3)) for k in range(121) for j in range(121)]
fit=find_fit(data,model)
fit

/usr/lib/python2.7/site-packages/scipy/optimize/minpack.py:427: RuntimeWarning:
Number of calls to function has reached maxfev = 3200.
  warnings.warn(errors[info][0], RuntimeWarning)
[a1 == (-7.69072654225465e-10),
 a10 == (-3.639376929901118e-08),
 a11 == (-5.433662796021851e-08),
 a12 == (-1.2527657633963957e-09),
 a13 == (1.784048647719785e-08),
 a14 == (-1.776884867225024e-08),
 a15 == (1.2690611241148885e-09),
 a2 == 0.0001303019595352706,
 a3 == 0.00013030293296301807,
 a4 == (-6.027627762127245e-06),
 a5 == (1.8085127469667956e-05),
 a6 == (1.735140302241286e-08),
 a7 == (3.387670800820787e-08),
 a8 == (1.6571083851957077e-08),
 a9 == (1.8003175475512318e-08)]
```

The previous warning is not serious as we will see.

```

modelf=model.substitute(fit)
print modelf
def green_model(z):
    w=z^(1/3)
    return modelf(w.real(),w.imag())

(x1, x2) |--> -(1.2527657633963957e-09)*x1^6 + (1.784048647719785e-08)*x1^4*x2^2 -
(1.776884867225024e-08)*x1^2*x2^4 + (1.2690611241148885e-09)*x2^6 +
(1.8003175475512318e-08)*x1^5 - (3.639376929901118e-08)*x1^3*x2^2 -
(5.433662796021851e-08)*x1*x2^4 + (1.735140302241286e-08)*x1^4 +
(3.387670800820787e-08)*x1^2*x2^2 + (1.6571083851957077e-08)*x2^4 -
(6.027627762127245e-06)*x1^3 + (1.8085127469667956e-05)*x1*x2^2 +
0.0001303019595352706*x1^2 + 0.00013030293296301807*x2^2 - (7.69072654225465e-10)*x1
- 0.748752485503338

a=random()
b=random()
z=2*a+1j*2*b
green(z)-green_model(z)
3.59554053197542e-10

```

The typical error of the approximation is  $5 \cdot 10^{-10}$ . So it is more than enough for our purposes.

```

timeit('green(z)')
25 loops, best of 3: 7.52 ms per loop

timeit('green_model(z)')
625 loops, best of 3: 342 micro-s per loop

```

The approximation is more than 20 times faster than the original function. We now adapt the optimization functions to use the approximation to the Green function.

```

def green_model_s(BB):
    z=BB[0]+I*BB[1]
    r=green_model(z)
    for j in range(len(AA)):
        p=small_pol[j][0]
        r=r-AA[j]*log(abs(p(z)))
    return r

def sup_pols_model(A):
    global AA
    if min(A)<0:
        return 10
    AA=A
    results=[]
    for z in seeds:
        x1=real(z)
        y1=imag(z)
        op=optimize.fmin(green_model_s, [x1,y1],disp=0)
        val=-green_model_s(op)
        results=results+[val]
    return max(results)

```

We now pick a collection of seeds distributed on the circle. Then we add each time a new polynomial to see if we can improve the lower bound and find more isolated values.

```

z1=exp(I*Pi/28)
z2=exp(I*6*Pi/35)
z3=exp(I*4*Pi/15)
z4=exp(I*8*Pi/21)
z5=exp(I*18*Pi/35)
z6=exp(I*23*Pi/35)
z7=exp(I*6*Pi/7)
seeds=[z1,z2,z3,z4,z5,z6,z7,-1]

```

```

AA=[7e-5]
coeffbound=[]
for j in range(23):
    a=optimize.fmin(sup_pols_model,AA,ftol=1e-10,disp=0)
    AA=list(a)
    b=sup_pols_model(AA)
    coeffbound=coeffbound+[[AA,-b]]
    print AA
    print 'newbound=',-b
    AA=AA+[0.]

[8.093750000000009e-05]
newbound= -0.748628177859874
[8.0839114671136495e-05, 6.0184048488736159e-06]
newbound= -0.748625170978969
[7.9768945318676147e-05, 4.4306227890180968e-06, 2.4498390472489291e-06]
newbound= -0.748623864986439
[7.8677969483938081e-05, 3.9831357582858071e-06, 2.6118301807463634e-06,
6.2316862940660201e-07]
newbound= -0.748623623472915
[7.7165309475827422e-05, 3.4571407512002551e-06, 2.1744072399931775e-06,
3.8335494017373395e-07, 3.940958544174513e-07]
newbound= -0.748623508652458
[7.727085234207566e-05, 3.4573038394512093e-06, 2.195738424273244e-06,
3.940169392577699e-07, 3.9928171696566594e-07, 7.2527404226696571e-08]
newbound= -0.748623455577464
[7.7271736389291246e-05, 3.4629400496233885e-06, 2.203626908773409e-06,
4.000349387590225e-07, 3.8204420526357151e-07, 7.4255980075422732e-08,
1.618519135160522e-08]
newbound= -0.748623445071868
[7.7272099559293265e-05, 3.462989472684365e-06, 2.2036315925750687e-06,
3.9999603613418961e-07, 3.8204076507653416e-07, 7.4264488215266521e-08,
1.6184357241110257e-08, 1.0342340969870803e-11]
newbound= -0.748623445029422
[7.7269934224023087e-05, 3.4642863999484197e-06, 2.1994215294872101e-06,
4.0031756529080831e-07, 3.8250694843556186e-07, 7.4275538780285349e-08,
1.6185890597712877e-08, 1.0826224539790258e-11, 5.0038335461923929e-10]
newbound= -0.748623444237185
[7.7269934224023087e-05, 3.4642863999484197e-06, 2.1994215294872101e-06,
4.0031756529080831e-07, 3.8250694843556186e-07, 7.4275538780285349e-08,
1.6185890597712877e-08, 1.1367535766779772e-11, 5.0038335461923929e-10, 0.0]
newbound= -0.748623444236888
[7.7269934224023087e-05, 3.4642863999484197e-06, 2.1994215294872101e-06,
4.0031756529080831e-07, 3.8250694843556186e-07, 7.4275538780285349e-08,
1.6185890597712877e-08, 1.193591255511876e-11, 5.0038335461923929e-10, 0.0, 0.0]
newbound= -0.748623444236575
[7.7269934224023087e-05, 3.4642863999484197e-06, 2.1994215294872101e-06,
4.0031756529080831e-07, 3.8250694843556186e-07, 7.4275538780285349e-08,
1.6185890597712877e-08, 1.2532708182874699e-11, 5.0038335461923929e-10, 0.0, 0.0,
0.0]
newbound= -0.748623444236247
[7.7269884619700119e-05, 3.4643605848868388e-06, 2.1993298463050131e-06,
4.0028856757218e-07, 3.8252683569091628e-07, 7.4276323788711715e-08,
1.6186084083384078e-08, 1.3157790367611487e-11, 5.0041907140216296e-10,
1.7752410988860616e-11, 1.4692075672376694e-11, 1.2243084529546056e-11,
1.0022667833366758e-11]
newbound= -0.748623444225311
[7.7269884619700119e-05, 3.4643605848868388e-06, 2.1993298463050131e-06,
4.0028856757218e-07, 3.8252683569091628e-07, 7.4276323788711715e-08,
1.6186084083384078e-08, 1.3157790367611487e-11, 5.0041907140216296e-10,
1.7752410988860616e-11, 1.5426679455995531e-11, 1.2243084529546056e-11,
1.0022667833366758e-11, 0.0]
newbound= -0.748623444224177
[7.7269884619700119e-05, 3.4643605848868388e-06, 2.1993298463050131e-06,

```

```

4.0028856757218e-07, 3.8252683569091628e-07, 7.4276323788711715e-08,
1.6186084083384078e-08, 1.3157790367611487e-11, 5.0041907140216296e-10,
1.7752410988860616e-11, 1.6198013428795307e-11, 1.2243084529546056e-11,
1.0022667833366758e-11, 0.0, 0.0]
newbound= -0.748623444222986
[7.7269884619700119e-05, 3.4643605848868388e-06, 2.1993298463050131e-06,
4.0028856757218e-07, 3.8252683569091628e-07, 7.4276323788711715e-08,
1.6186084083384078e-08, 1.3157790367611487e-11, 5.0041907140216296e-10,
1.7752410988860616e-11, 1.7007914100235074e-11, 1.2243084529546056e-11,
1.0022667833366758e-11, 0.0, 0.0, 0.0]
newbound= -0.748623444221736
[7.7269884619700119e-05, 3.4643605848868388e-06, 2.1993298463050131e-06,
4.0028856757218e-07, 3.8252683569091628e-07, 7.4276323788711715e-08,
1.6186084083384078e-08, 1.3157790367611487e-11, 5.0041907140216296e-10,
1.7752410988860616e-11, 1.7858309805246826e-11, 1.2243084529546056e-11,
1.0022667833366758e-11, 0.0, 0.0, 0.0, 0.0]
newbound= -0.748623444220423
[7.7269884619700119e-05, 3.4643605848868388e-06, 2.1993298463050131e-06,
4.0028856757218e-07, 3.8252683569091628e-07, 7.4276323788711715e-08,
1.6186084083384078e-08, 1.3157790367611487e-11, 5.0041907140216296e-10,
1.800292108533428e-11, 1.7993031917791291e-11, 1.2590111412817611e-11,
1.0022667833366758e-11, 0.0, 0.0, 0.0, 0.0, 0.0]
newbound= -0.748623444219663
[7.7269884619700119e-05, 3.4643605848868388e-06, 2.1993298463050131e-06,
4.0028856757218e-07, 3.8252683569091628e-07, 7.4276323788711715e-08,
1.6186084083384078e-08, 1.3157790367611487e-11, 5.0041907140216296e-10,
1.8903067139600994e-11, 1.7993031917791291e-11, 1.2590111412817611e-11,
1.0022667833366758e-11, 0.0, 0.0, 0.0, 0.0, 0.0, 0.0]
newbound= -0.748623444219442
[7.7269884619700119e-05, 3.4643605848868388e-06, 2.1993298463050131e-06,
4.0028856757218e-07, 3.8252683569091628e-07, 7.4276323788711715e-08,
1.6186084083384078e-08, 1.3157790367611487e-11, 5.0041907140216296e-10,
1.9848220496581044e-11, 1.7993031917791291e-11, 1.2590111412817611e-11,
1.0022667833366758e-11, 0.0, 0.0, 0.0, 0.0, 0.0, 0.0, 0.0, 0.0]
newbound= -0.748623444219211
[7.7269884619700119e-05, 3.4643605848868388e-06, 2.1993298463050131e-06,
4.0028856757218e-07, 3.8252683569091628e-07, 7.4276323788711715e-08,
1.6186084083384078e-08, 1.3157790367611487e-11, 5.0041907140216296e-10,
2.0840631521410099e-11, 1.7993031917791291e-11, 1.2590111412817611e-11,
1.0022667833366758e-11, 0.0, 0.0, 0.0, 0.0, 0.0, 0.0, 0.0, 0.0]
newbound= -0.748623444218968
[7.7269884619700119e-05, 3.4643605848868388e-06, 2.1993298463050131e-06,
4.0028856757218e-07, 3.8252683569091628e-07, 7.4276323788711715e-08,
1.6186084083384078e-08, 1.3157790367611487e-11, 5.0041907140216296e-10,
2.1882663097480604e-11, 1.7993031917791291e-11, 1.2590111412817611e-11,
1.0022667833366758e-11, 0.0, 0.0, 0.0, 0.0, 0.0, 0.0, 0.0, 0.0, 0.0]
newbound= -0.748623444218712
[7.7269873460609296e-05, 3.4643538741983628e-06, 2.1993181318410657e-06,
4.0028718718475536e-07, 3.8252619168785997e-07, 7.4276209787094527e-08,
1.6186093950749018e-08, 1.3157864272032226e-11, 5.0042116216257335e-10,
2.2976384917766112e-11, 1.7993132980702613e-11, 1.2590182128710254e-11,
1.0022724128492295e-11, 1.2301740977939008e-13, 1.9469820281465363e-13,
1.8121521708028825e-13, 1.552952094482885e-13, 6.5087576146211706e-13,
1.0672026649989196e-13, 4.6957809024850328e-13, 1.4352482717572456e-13,
1.6792121330359753e-13, 1.1692629467480607e-13]
newbound= -0.748623444218005

```

As we can see, adding up to 7 polynomials improves slightly the lower bound of the essential minimum. But adding more than 7 polynomials has almost no effect on the lower bound. Moreover, even adding more than 20 polynomials we are not able to prove that the next value of the height is isolated. In conclusion we have the following experimental distribution of the Faltings height of elliptic curves.

**Isolated values:**  $h(\infty) = -\infty$ ,  $h(0) = -.74875248$ ,  $h(1) = -.74862817$ ,  $h(\rho) = -.74862517$ ,  $h(z_1) = -.74862366$ , where  $\rho$  is a root of the polynomial  $t^2 - t + 1$  and  $z_1$  is a root of  $t^4 - t^3 + t^2 - t + 1$ .

**Lower bound** of the essential minimum:  $-.74862344$ .

Next known value:  $-.74862330$ .

**Upper bound:**  $-.74862278$ .

Indeterminacy of the essential minimum:  $< 10^{-6}$ .

Between  $-.74862278$  and  $\infty$  there are no gaps. The values of the height are dense on this interval.

## References

[BMRL]      José Burgos Gil, Ricardo Menares and Juan Rivera-Letelier. On the essential minimum of Faltings' height.

José Ignacio Burgos Gil. Instituto de Ciencias Matemáticas (CSIC-UAM-UCM-UCM3). Calle Nicolás Cabrera 15, Campus UAB, Cantoblanco, 28049 Madrid, Spain  
`burgos@icmat.es`  
<http://www.icmat.es/miembros/burgos>

Ricardo Menares. Instituto de Matemáticas, Pontificia Universidad Católica de Valparaíso, Blanco Viel 596, Cerro Barón, Valparaíso, Chile.  
`ricardo.menares@pucv.cl`  
<http://ima.ucv.cl/academico/ricardo-menares/>

Juan Rivera-Letelier. Department of Mathematics, University of Rochester. Hylan Building, Rochester, NY 14627, U.S.A.  
`riveraletelier@gmail.com`  
<http://rivera-letelier.org>
